# Supplementary material for: The 2025 Foundation Model Transparency Index
Source: arXiv:2512.10169 source file (2025-12-11)
Supplement: Supplementary file 1 [file app_selection.tex]

\hypertarget{selection}{\section{Selection decisions}}
\label{app:selection}

In conducting the index, core structural design decisions are (i) the indicators used to assess developers and (ii) the developers that are assessed.
Here, we clarify both matters.
\subsection{Indicator selection}
\label{app:indicator-selection}
We use the same 100 indicators as FMTI v1.0 to facilitate direct comparison.
These indicators are listed by domain in \autoref{fig:indicators}.

\subsection{Developer selection}
\label{app:developer-selection}
We contacted 19 foundation model developers to request these developers submit transparency reports for the purpose of conducting FMTI v1.1.
Consistent with the principles used by \citet{bommasani2023fmti}, we only considered developers that are companies and that develop prominent foundation models.
Specifically, we contacted leadership via email at 01.ai, Adept, AI21 Labs, Aleph Alpha, Amazon, Anthropic, BigCode (Hugging Face and ServiceNow), Cohere, Databricks, Google, IBM, Inflection, Meta, Microsoft, Mistral, OpenAI, Stability AI, Writer, and xAI.
Following this email correspondence, and further clarification of the nature of the request, 14 foundation model developers agreed to provide the requested transparency reports.

Therefore, our selection process deliberately excluded foundation model developers that are not companies, even if they develop prominent foundation models, such as the Allen Institute for AI \citep[developer of models such as OLMo;][]{groeneveld2024olmo} and EleutherAI \citep[developer of Pythia;][]{biderman2023pythia}.
While developers such as AI2 and EleutherAI are often leaders in various types of transparency, releasing detailed information about data \citep{gao2020pile, soldaini2024dolma}, evaluations \citep{gao2021framework, magnusson2023paloma}, and the model development pipeline \citep{black2022neox, biderman2023pythia, groeneveld2024olmo}, we consider only companies in selecting developers to assess in FMTI v1.1. 

Our selection process also did not involve engagement with developers where we lacked connections with their leadership, which often coincides with models developed outside the United States and the Western hemisphere (\eg the developers of Falcon \citep{almazrouei2023falcon}, Qwen \citep{bai2023qwen}, DeepSeek \citep{deepseekai2024deepseek}, and HyperCLOVA \citep{yoo2024hyperclova}).

Finally, we did not engage any developer that released its first prominent foundation model during our execution of FMTI v1.1 (such releases include Apple's MM1 \citep{mckinzie2024mm1}, SambaNova's Samba 1 \citep{samba1}, Reka's Reka Core \citep{rekateam2024reka}, and Snowflake's Arctic-1 \citep{merrick2024arcticembed}). 
Moving forward, having successfully demonstrated that prominent foundation model developers have cooperated by submitting transparency reports, subsequent versions of the Foundation Model Transparency Index may engage these companies as well as others.
